# Supplementary material for: ColdGuess: A General and Effective Relational Graph Convolutional Network to Tackle Cold Start Cases
Source: arXiv:2205.12318 source file (2022-05-26)
Supplement: Supplementary file 1 [file appendix.tex]

\section*{Appendix}
% \subsection*{Label Distribution}
% Figure~\ref{fig:label_dist} shows the label distribution. Figure~\ref{fig:new_seller} shows the proportion of complaints contributed by new sellers. Both plots are based on train data as of 2020/10. 

% \begin{figure}[h]
% \centering
%   \includegraphics[scale=0.6]{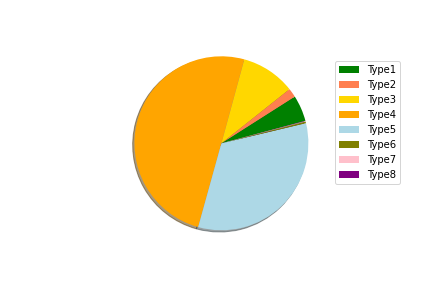}
% \caption{Number of offers in each complaint type}
% \label{fig:label_dist}
% \end{figure}

% \begin{figure}[h]
% \centering
%   \includegraphics[scale=0.48]{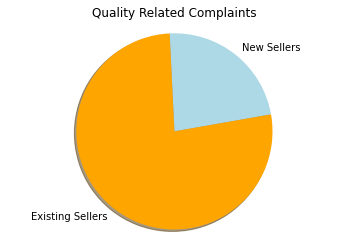}
% \caption{Proportion of complaints contributed by new sellers}
% \label{fig:new_seller}
% \end{figure}

\subsection*{A Summary of Train and Test Data Sets}
% Table~\ref{tab:dataset} gives an overview of test sets (from 2020/11 to 2021/04). %Train set has twice as much data as test sets because of the Prime Day happening in 2020/10 and thus higher volume. 
Table~\ref{tab:dataset} gives an overview of test sets over six months.
\begin{table}[h]
\begin{threeparttable}
 \caption{A summary of Seller-\ASINg graphs built on test sets. We show the percentage of new offer edges, new seller nodes and new ASIN nodes simulated in each month.}
\label{tab:dataset}
 \centering
\begin{tabular}{lrrr}
 \toprule 
\cmidrule(r){1-4}
\hline
  Month   & \% of new    & \% of new     & \% of new \\
          &  offer edges & seller nodes  &  \ASIN nodes \\
\hline
%   2020/11   &  25.26\%  &  12.84\%  &  3.95\%   \\
%   2020/12   &  25.57\%  &  13.00\%  &  4.01\%   \\
%   2021/01   &  25.68\%  &  12.94\%  &  4.02\%   \\
%   2021/02   &  25.50\%  &  12.87\%  &  4.05\%   \\
%   2021/03   &  19.85\%  &  10.02\%  &  3.70\%   \\
%   2021/04	&  26.65\%	&  13.32\%	&  4.28\%   \\
  month1   &  25.26\%  &  12.84\%  &  3.95\%   \\
  month2   &  25.57\%  &  13.00\%  &  4.01\%   \\
  month3   &  25.68\%  &  12.94\%  &  4.02\%   \\
  month4   &  25.50\%  &  12.87\%  &  4.05\%   \\
  month5   &  19.85\%  &  10.02\%  &  3.70\%   \\
  month6   &  26.65\%  &  13.32\%	&  4.28\%   \\
\hline
% \bottomrule
\end{tabular}
\begin{tablenotes}
    \small
%  \item Train set is 2020/10. Test sets are from 2020/11 to 2021/04. We simulated cold start scenarios only for test sets. %The train set has twice as much data as test sets because the train set is in prime month and has higher volumes. 
  \item We simulated cold start scenarios only for test sets, not train set.
 \end{tablenotes}
 \end{threeparttable}
% this is metioned in 4.1.2
\end{table}

\subsection*{Performance comparison among \pcdetector, Graph+LGBM, and LGBM}

\paragraph{Full spectrum of sample data} Table~\ref{tab:results-origin} (corresponds to top left plots from Figure~\ref{fig:202101} to Figure~\ref{fig:202104}) shows that \pcdetector has close performance with LGBM in all 9 classes when being evaluated on full data sets.

\paragraph{New offer case} Table~\ref{tab:results-newoffer}(corresponds to top right plots from Figure~\ref{fig:202101} to Figure~\ref{fig:202104}) compares the performance of \pcdetector, LGBM, and Graph+LGBM on new offers. In this case, we assigned the offer features to missing values except the list price. It results in 104 missing offer edge features. We found that Graph+LGBM outperforms LGBM in all classes except \OtherNPE by 0.4-7\% absolute AUC, \method outperforms LGBM in all 9 except \USN by 1-9\% absolute AUC, and \method outperforms Graph+LGBM in 7 out of 9 classes except \USN and \CCR by up to 1.9\% absolute AUC . 

\paragraph{New seller case} Table~\ref{tab:results-newseller}(corresponds to bottom left plots from Figure~\ref{fig:202101} to Figure~\ref{fig:202104}) compares the performance of \pcdetector, LGBM, and Graph+LGBM on new sellers. In this case, we assigned both the offer and seller features to missing values except list price. It results in 160 missing features in total. We found hat \pcdetector outperforms LGBM in all classes by 1.4-20.6\% absolute AUC, and \pcdetector outperforms Graph+LGBM in all classes except \USN by 1.5-11.9\% absolute AUC.

\paragraph{New seller sells a new ASIN case} Table~\ref{tab:results-newasin-2} (corresponds to bottom right plots from Figure~\ref{fig:202101} to Figure~\ref{fig:202104}) compares the performance of \pcdetector and LGBM on new sellers who created a new ASIN case. In this case, we assigned offer, seller, and ASIN features to missing values except offer price and ASIN GL group because these two features are known once an offer is created. With only two available features, \pcdetector outperforms LGBM in all classes by \textbf{12-35\%}, \pcdetector outperforms Graph+LGBM in all classes by \textbf{7.1-34\%}.

\begin{table*}
\begin{threeparttable}
 \caption{\method vs. LGBM vs. Graph+LGBM ROC-AUC on the full spectrum of data using $G_o$. We take LGBM as the baseline model and present relative ROC-AUC improvement from Graph+LGBM and \method}
\label{tab:results-origin}
 \centering
\begin{tabular}{lrrrrrrrrr}
 \toprule 
\cmidrule(r){1-4}
\hline
%   Month   & WIS &  USN &  Damaged & Other NPE  & Defective  &
%           VM   & CCR  & EPCR & Normal\\
  Month   & \WIS &  \USN &  \Damaged &  \OtherNPE  & \Defective  &
          \VM    &  \CCR &  \EPCR    & Normal\\
\hline
\multicolumn{10}{c}{Graph-LGBM} \\
\hline
% Nov-20 & 0.58\% & 0.28\% & -0.02\% & -0.01\% & -0.07\% & 1.33\% & 1.30\% & 0.93\% & -0.06\% \\
% Dec-20 & 0.41\% & 0.30\% & 0.00\% & 0.02\% & -0.04\% & 1.47\% & 1.38\% & 0.92\% & -0.06\% \\
% Jan-21 & 0.67\% & 0.42\% & 0.10\% & 0.10\% & 0.01\% & 1.40\% & 2.08\% & 2.45\% & 0.09\% \\
% Feb-21 & 0.60\% & 0.50\% & 0.04\% & 0.10\% & 0.01\% & 1.39\% & 2.77\% & 2.66\% & 0.06\% \\
% Mar-21 & 0.45\% & 0.28\% & 0.06\% & 0.13\% & 0.05\% & 0.79\% & 2.09\% & 3.82\% & 0.13\% \\
% Apr-21 & 0.22\% & 0.31\% & 0.01\% & 0.05\% & -0.06\% & 0.80\% & 1.58\% & 1.12\% & -0.08\% \\

Month1 & 0.58\% & 0.28\% & -0.02\% & -0.01\% & -0.07\% & 1.33\% & 1.30\% & 0.93\% & -0.06\% \\
Month2  & 0.41\% & 0.30\% & 0.00\% & 0.02\% & -0.04\% & 1.47\% & 1.38\% & 0.92\% & -0.06\% \\
Month3 & 0.67\% & 0.42\% & 0.10\% & 0.10\% & 0.01\% & 1.40\% & 2.08\% & 2.45\% & 0.09\% \\
Month4  & 0.60\% & 0.50\% & 0.04\% & 0.10\% & 0.01\% & 1.39\% & 2.77\% & 2.66\% & 0.06\% \\
Month5  & 0.45\% & 0.28\% & 0.06\% & 0.13\% & 0.05\% & 0.79\% & 2.09\% & 3.82\% & 0.13\% \\
Month6  & 0.22\% & 0.31\% & 0.01\% & 0.05\% & -0.06\% & 0.80\% & 1.58\% & 1.12\% & -0.08\% \\

\hline
\multicolumn{10}{c}{\pcdetector} \\
\hline
% Nov-20 & 0.15\% & -0.16\% & -0.22\% & -0.26\% & -0.09\% & 1.54\% & -0.13\% & 1.21\% & -0.39\% \\
% Dec-20 & 0.13\% & 0.10\% & -0.17\% & -0.30\% & -0.09\% & 1.66\% & 0.39\% & 1.85\% & -0.40\% \\
% Jan-21 & 0.18\% & 0.26\% & -0.15\% & -0.17\% & -0.12\% & 1.04\% & -0.56\% & 3.05\% & -0.23\% \\
% Feb-21 & 0.17\% & 0.10\% & -0.24\% & -0.12\% & -0.14\% & 0.92\% & 0.52\% & 3.76\% & -0.35\% \\
% Mar-21 & -0.01\% & -0.27\% & -0.22\% & 0.31\% & -0.30\% & -0.42\% & 0.24\% & 3.90\% & -0.31\% \\
% Apr-21 & -0.20\% & -0.08\% & -0.14\% & -0.30\% & -0.11\% & 0.83\% & 0.07\% & 1.46\% & -0.36\% \\
Month1 & 0.15\% & -0.16\% & -0.22\% & -0.26\% & -0.09\% & 1.54\% & -0.13\% & 1.21\% & -0.39\% \\
Month2 & 0.13\% & 0.10\% & -0.17\% & -0.30\% & -0.09\% & 1.66\% & 0.39\% & 1.85\% & -0.40\% \\
Month3 & 0.18\% & 0.26\% & -0.15\% & -0.17\% & -0.12\% & 1.04\% & -0.56\% & 3.05\% & -0.23\% \\
Month4 & 0.17\% & 0.10\% & -0.24\% & -0.12\% & -0.14\% & 0.92\% & 0.52\% & 3.76\% & -0.35\% \\
Month5 & -0.01\% & -0.27\% & -0.22\% & 0.31\% & -0.30\% & -0.42\% & 0.24\% & 3.90\% & -0.31\% \\
Month6 & -0.20\% & -0.08\% & -0.14\% & -0.30\% & -0.11\% & 0.83\% & 0.07\% & 1.46\% & -0.36\% \\
\hline
% \bottomrule
\end{tabular}
\end{threeparttable}
\end{table*}

\begin{table*}
\begin{threeparttable}
 \caption{\method vs. LGBM vs. Graph+LGBM ROC-AUC on new offer samples using $G_{no}$. We take LGBM as the baseline model and present relative ROC-AUC improvement from Graph+LGBM and \method.}
\label{tab:results-newoffer}
 \centering
\begin{tabular}{lrrrrrrrrr}
 \toprule 
\cmidrule(r){1-4}
\hline
%   Month   & WIS &  USN &  Damaged & Other NPE  & Defective  &
%           VM   & CCR  & EPCR & Normal\\
  Month   & \WIS &  \USN &  \Damaged &  \OtherNPE  & \Defective  &
          \VM    &  \CCR &  \EPCR    & Normal\\
\hline
\multicolumn{10}{c}{Graph+LGBM} \\
\hline
% Nov-20 & 5.18\% & 0.73\% & 0.64\% & -0.10\% & 0.29\% & 2.37\% & 2.75\% & 1.35\% & 0.21\% \\
% Dec-20 & 3.92\% & 0.68\% & 0.88\% & -0.33\% & 0.20\% & 2.18\% & 2.62\% & 1.98\% & 0.15\% \\
% Jan-21 & 4.42\% & 0.78\% & 0.85\% & -0.42\% & 0.41\% & 1.74\% & 4.10\% & 3.37\% & 0.41\% \\
% Feb-21 & 4.44\% & 1.09\% & 1.28\% & -0.03\% & 0.48\% & 2.23\% & 3.66\% & 3.42\% & 0.37\% \\
% Mar-21 & 3.35\% & 0.34\% & 0.96\% & -0.28\% & 0.34\% & 1.11\% & 3.61\% & 9.17\% & 0.63\% \\
% Apr-21 & 2.27\% & 0.75\% & 0.82\% & -0.14\% & 0.36\% & 0.63\% & 1.62\% & 1.78\% & 0.36\% \\
Month1 & 5.18\% & 0.73\% & 0.64\% & -0.10\% & 0.29\% & 2.37\% & 2.75\% & 1.35\% & 0.21\% \\
Month2 & 3.92\% & 0.68\% & 0.88\% & -0.33\% & 0.20\% & 2.18\% & 2.62\% & 1.98\% & 0.15\% \\
Month3 & 4.42\% & 0.78\% & 0.85\% & -0.42\% & 0.41\% & 1.74\% & 4.10\% & 3.37\% & 0.41\% \\
Month4 & 4.44\% & 1.09\% & 1.28\% & -0.03\% & 0.48\% & 2.23\% & 3.66\% & 3.42\% & 0.37\% \\
Month5 & 3.35\% & 0.34\% & 0.96\% & -0.28\% & 0.34\% & 1.11\% & 3.61\% & 9.17\% & 0.63\% \\
Month6 & 2.27\% & 0.75\% & 0.82\% & -0.14\% & 0.36\% & 0.63\% & 1.62\% & 1.78\% & 0.36\% \\
\hline
\multicolumn{10}{c}{\pcdetector} \\
\hline
% Nov-20 & 6.36\% & -1.17\% & 1.24\% & 1.38\% & 1.68\% & 3.45\% & 1.10\% & 0.92\% & 1.20\% \\
% Dec-20 & 5.15\% & -0.45\% & 1.31\% & 1.11\% & 1.66\% & 2.69\% & 1.66\% & 2.94\% & 1.32\% \\
% Jan-21 & 5.47\% & -0.41\% & 1.09\% & 1.12\% & 1.61\% & 1.72\% & 1.93\% & 4.34\% & 1.45\% \\
% Feb-21 & 5.81\% & 0.11\% & 1.83\% & 1.74\% & 2.01\% & 2.23\% & 2.03\% & 5.13\% & 1.57\% \\
% Mar-21 & 3.67\% & -0.94\% & 1.31\% & 1.07\% & 1.69\% & 1.63\% & 1.91\% & 7.79\% & 1.86\% \\
% Apr-21 & 3.03\% & -0.57\% & 2.02\% & 1.32\% & 1.97\% & 1.62\% & 0.85\% & 2.93\% & 1.54\% \\

Month1 & 6.36\% & -1.17\% & 1.24\% & 1.38\% & 1.68\% & 3.45\% & 1.10\% & 0.92\% & 1.20\% \\
Month2 & 5.15\% & -0.45\% & 1.31\% & 1.11\% & 1.66\% & 2.69\% & 1.66\% & 2.94\% & 1.32\% \\
Month3 & 5.47\% & -0.41\% & 1.09\% & 1.12\% & 1.61\% & 1.72\% & 1.93\% & 4.34\% & 1.45\% \\
Month4 & 5.81\% & 0.11\% & 1.83\% & 1.74\% & 2.01\% & 2.23\% & 2.03\% & 5.13\% & 1.57\% \\
Month5 & 3.67\% & -0.94\% & 1.31\% & 1.07\% & 1.69\% & 1.63\% & 1.91\% & 7.79\% & 1.86\% \\
Month6 & 3.03\% & -0.57\% & 2.02\% & 1.32\% & 1.97\% & 1.62\% & 0.85\% & 2.93\% & 1.54\% \\
\hline
% \bottomrule
\end{tabular}
\begin{tablenotes}
      \small
      \item[a] The AUC difference between \method and LGBM greater than 1 pcp is gray bolded; AUC difference greater than 5 pcp is black bolded. 
\end{tablenotes}
\end{threeparttable}
\end{table*}

\begin{table*}
\begin{threeparttable}
 \caption{\method vs. LGBM vs. Graph+LGBM ROC-AUC on new seller sample using $G_{ns}$. We take LGBM as the baseline model and present relative ROC-AUC improvement from Graph+LGBM and \method.}
\label{tab:results-newseller}
 \centering
\begin{tabular}{lrrrrrrrrr}
 \toprule 
\cmidrule(r){1-4}
\hline
%   Month   & WIS &  USN &  Damaged & Other NPE  & Defective  &
%           VM   & CCR  & EPCR & Normal\\
  Month   & \WIS &  \USN &  \Damaged &  \OtherNPE  & \Defective  &
          \VM    &  \CCR &  \EPCR    & Normal\\
\hline
\multicolumn{10}{c}{Graph+LGBM} \\
\hline
% Nov-20 & 5.42\% & 3.53\% & 0.50\% & 0.56\% & 1.73\% & 5.73\% & 0.03\% & 3.53\% & 0.22\% \\
% Dec-20 & 4.87\% & 3.97\% & 0.85\% & 0.40\% & 1.69\% & 4.00\% & 3.58\% & 3.65\% & 0.32\% \\
% Jan-21 & 4.49\% & 4.04\% & 0.76\% & 0.43\% & 2.00\% & 2.47\% & 4.55\% & 8.25\% & -0.17\% \\
% Feb-21 & 4.99\% & 4.11\% & 0.98\% & 0.82\% & 2.28\% & 2.43\% & 7.32\% & 6.27\% & 0.23\% \\
% Mar-21 & 5.19\% & 3.16\% & 1.10\% & -0.02\% & 2.74\% & 2.86\% & 7.20\% & 9.62\% & 0.43\% \\
% Apr-21 & 2.78\% & 3.14\% & 1.07\% & 0.97\% & 2.39\% & 1.02\% & 6.12\% & 3.30\% & 1.06\% \\
Month1 & 5.42\% & 3.53\% & 0.50\% & 0.56\% & 1.73\% & 5.73\% & 0.03\% & 3.53\% & 0.22\% \\
Month2 & 4.87\% & 3.97\% & 0.85\% & 0.40\% & 1.69\% & 4.00\% & 3.58\% & 3.65\% & 0.32\% \\
Month3 & 4.49\% & 4.04\% & 0.76\% & 0.43\% & 2.00\% & 2.47\% & 4.55\% & 8.25\% & -0.17\% \\
Month4 & 4.99\% & 4.11\% & 0.98\% & 0.82\% & 2.28\% & 2.43\% & 7.32\% & 6.27\% & 0.23\% \\
Month5 & 5.19\% & 3.16\% & 1.10\% & -0.02\% & 2.74\% & 2.86\% & 7.20\% & 9.62\% & 0.43\% \\
Month6 & 2.78\% & 3.14\% & 1.07\% & 0.97\% & 2.39\% & 1.02\% & 6.12\% & 3.30\% & 1.06\% \\
\hline
\multicolumn{10}{c}{\pcdetector} \\
\hline
% Nov-20 & 6.43\% & 2.19\% & 2.34\% & 3.09\% & 4.50\% & 11.24\% & 12.32\% & 5.18\% & 5.85\% \\
% Dec-20 & 5.90\% & 2.73\% & 2.77\% & 2.81\% & 4.82\% & 9.47\% & 14.61\% & 7.00\% & 6.30\% \\
% Jan-21 & 5.21\% & 3.07\% & 2.73\% & 2.56\% & 4.89\% & 8.01\% & 12.37\% & 12.39\% & 6.30\% \\
% Feb-21 & 6.23\% & 2.90\% & 3.11\% & 3.50\% & 5.52\% & 7.07\% & 15.13\% & 12.85\% & 7.40\% \\
% Mar-21 & 5.37\% & 0.47\% & 1.21\% & 1.07\% & 5.20\% & 6.93\% & 13.26\% & 12.52\% & 7.49\% \\
% Apr-21 & 3.19\% & 2.53\% & 2.85\% & 2.64\% & 5.04\% & 7.65\% & 14.64\% & 8.79\% & 6.02\% \\
Month1 & 6.43\% & 2.19\% & 2.34\% & 3.09\% & 4.50\% & 11.24\% & 12.32\% & 5.18\% & 5.85\% \\
Month2 & 5.90\% & 2.73\% & 2.77\% & 2.81\% & 4.82\% & 9.47\% & 14.61\% & 7.00\% & 6.30\% \\
Month3 & 5.21\% & 3.07\% & 2.73\% & 2.56\% & 4.89\% & 8.01\% & 12.37\% & 12.39\% & 6.30\% \\
Month4 & 6.23\% & 2.90\% & 3.11\% & 3.50\% & 5.52\% & 7.07\% & 15.13\% & 12.85\% & 7.40\% \\
Month5 & 5.37\% & 0.47\% & 1.21\% & 1.07\% & 5.20\% & 6.93\% & 13.26\% & 12.52\% & 7.49\% \\
Month6 & 3.19\% & 2.53\% & 2.85\% & 2.64\% & 5.04\% & 7.65\% & 14.64\% & 8.79\% & 6.02\% \\
\hline
% \bottomrule
\end{tabular}
\begin{tablenotes}
      \small
      \item[a] The AUC difference between \method and LGBM greater than 1 pcp is gray bolded; AUC difference greater than 5 pcp is black bolded. 
\end{tablenotes}
\end{threeparttable}
\end{table*}

\begin{table*}
\begin{threeparttable}
 \caption{\method vs. LGBM vs. Graph+LGBM ROC-AUC on new Sellers sell new ASIN case using $G_{nsna}$.We take LGBM as the baseline model and present relative ROC-AUC improvement from Graph+LGBM and \method.}
\label{tab:results-newasin-2}
 \centering
\begin{tabular}{lrrrrrrrrr}
 \toprule 
\cmidrule(r){1-4}
\hline
%   Month   & WIS &  USN &  Damaged &  Other NPE  & Defective  &
%           VM    &  CCR &  EPCR    & Normal\\
  Month   & \WIS &  \USN &  \Damaged &  \OtherNPE  & \Defective  &
          \VM    &  \CCR &  \EPCR    & Normal\\
\hline
\multicolumn{10}{c}{Graph+LGBM} \\
\hline
% Nov-20 & 5.25\% & 6.22\% & 0.48\% & 2.41\% & -0.05\% & 3.22\% & 1.19\% & 0.91\% & -0.68\% \\
% Dec-20 & 4.73\% & 6.42\% & 0.66\% & 2.23\% & 0.03\% & 2.81\% & 2.08\% & 0.25\% & -0.87\% \\
% Jan-21 & 5.13\% & 6.40\% & 0.56\% & 2.62\% & -0.07\% & 3.81\% & 1.35\% & 0.37\% & -0.93\% \\
% Feb-21 & 4.52\% & 6.20\% & 0.58\% & 2.15\% & 0.10\% & 3.36\% & 3.23\% & 1.39\% & -0.79\% \\
% Mar-21 & 6.42\% & 3.83\% & 0.76\% & 1.34\% & 0.49\% & 0.09\% & -0.55\% & 2.13\% & -1.10\% \\
% Apr-21 & 2.09\% & 3.98\% & 0.70\% & 2.05\% & 0.26\% & 0.26\% & 0.84\% & 5.86\% & -0.22\% \\

Month1 & 5.25\% & 6.22\% & 0.48\% & 2.41\% & -0.05\% & 3.22\% & 1.19\% & 0.91\% & -0.68\% \\
Month2 & 4.73\% & 6.42\% & 0.66\% & 2.23\% & 0.03\% & 2.81\% & 2.08\% & 0.25\% & -0.87\% \\
Month3 & 5.13\% & 6.40\% & 0.56\% & 2.62\% & -0.07\% & 3.81\% & 1.35\% & 0.37\% & -0.93\% \\
Month4 & 4.52\% & 6.20\% & 0.58\% & 2.15\% & 0.10\% & 3.36\% & 3.23\% & 1.39\% & -0.79\% \\
Month4 & 6.42\% & 3.83\% & 0.76\% & 1.34\% & 0.49\% & 0.09\% & -0.55\% & 2.13\% & -1.10\% \\
Month5 & 2.09\% & 3.98\% & 0.70\% & 2.05\% & 0.26\% & 0.26\% & 0.84\% & 5.86\% & -0.22\% \\
\hline
\multicolumn{10}{c}{\pcdetector} \\
\hline
Month1 & 17.77\% & 16.19\% & 13.82\% & 13.48\% & 9.54\% & 12.73\% & 34.09\% & 11.85\% & 23.22\% \\
Month2 & 17.57\% & 15.86\% & 14.62\% & 12.94\% & 10.11\% & 12.93\% & 33.74\% & 12.75\% & 23.78\% \\
Month3 & 17.29\% & 16.62\% & 14.63\% & 12.78\% & 9.76\% & 14.52\% & 33.02\% & 14.97\% & 22.91\% \\
Month4 & 17.50\% & 16.50\% & 15.49\% & 12.46\% & 10.04\% & 15.07\% & 36.02\% & 16.66\% & 25.36\% \\
Month5 & 16.81\% & 14.69\% & 13.92\% & 8.13\% & 9.36\% & 15.07\% & 33.47\% & 9.39\% & 24.01\% \\
Month6 & 16.31\% & 17.95\% & 13.98\% & 11.89\% & 8.91\% & 11.69\% & 34.97\% & 13.93\% & 24.24\% \\
\hline
% \bottomrule
\end{tabular}
\begin{tablenotes}
      \small
      \item[a] The AUC difference between \method and LGBM greater than 5 pcp is black bolded. 
\end{tablenotes}
\end{threeparttable}
\end{table*}

\subsection*{\method vs. LGBM vs. Graph+LGBM Evaluation from 2020/12 to 2021/4}

\begin{figure*}
    \includegraphics[width=.35\textwidth]{Figures/2020-12_All Data.png}\hfill
    \includegraphics[width=.35\textwidth]{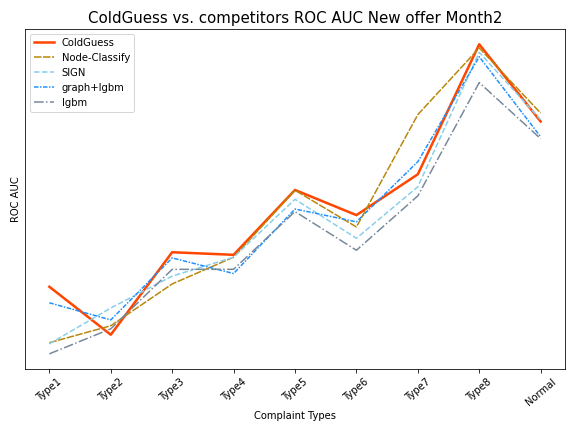}\hfill
    \\[\smallskipamount]
    \includegraphics[width=.35\textwidth]{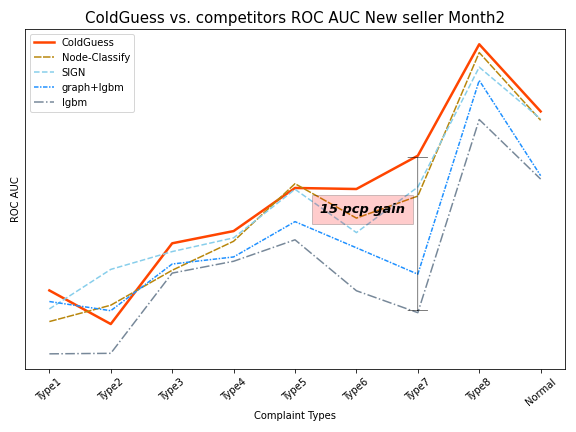}\hfill
    \includegraphics[width=.35\textwidth]{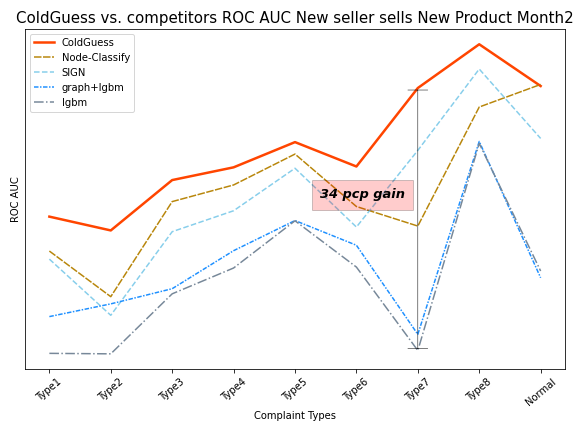}\hfill
    \caption{\method vs. LGBM vs. Graph+LGBM on a full spectrum of sample data (top left), new offer case (top right), new seller case (bottom left), and new seller sell new \ASIN case (bottom right) using data of Month2.}
    \label{fig:202012}
\end{figure*}

\begin{figure*}
    \includegraphics[width=.35\textwidth]{Figures/2021-01_All Data.png}\hfill
    \includegraphics[width=.35\textwidth]{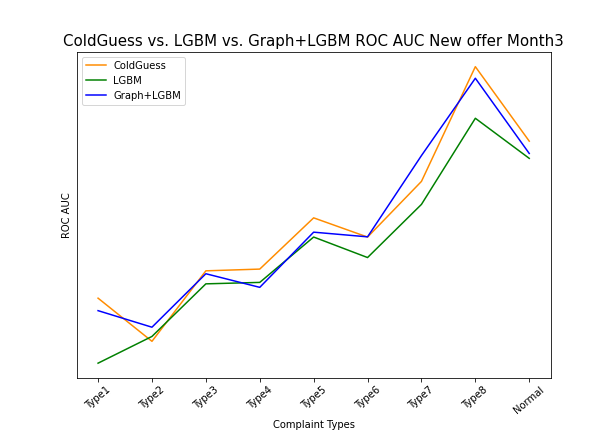}\hfill
    \\[\smallskipamount]
    \includegraphics[width=.35\textwidth]{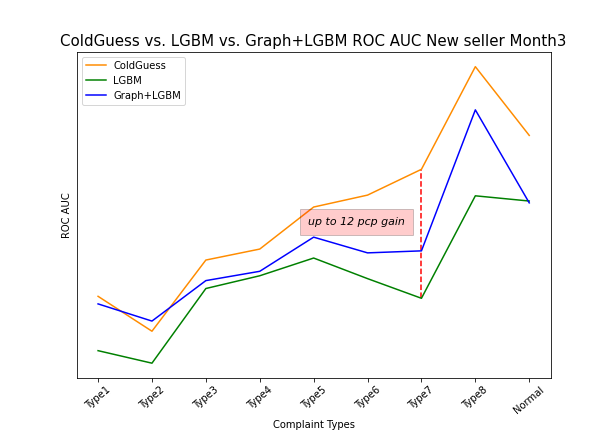}\hfill
    \includegraphics[width=.35\textwidth]{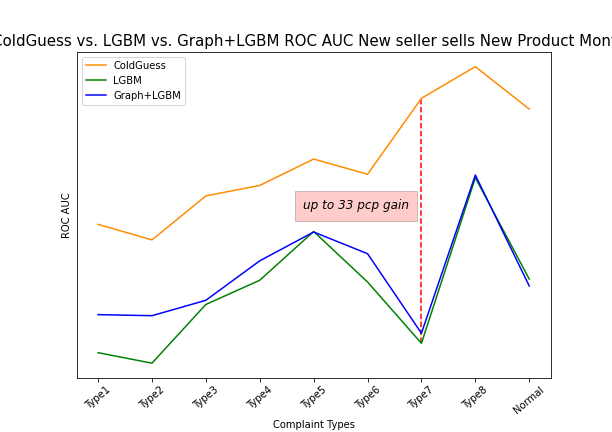}\hfill
    \caption{\method vs. LGBM vs. Graph+LGBM on a full spectrum of sample data (top left), new offer case (top right), new seller case (bottom left), and new seller sell new \ASIN case (bottom right) using data of Month3.}
    \label{fig:202101}
\end{figure*}

\begin{figure*}
    \includegraphics[width=.35\textwidth]{Figures/2021-02_All Data.png}\hfill
    \includegraphics[width=.35\textwidth]{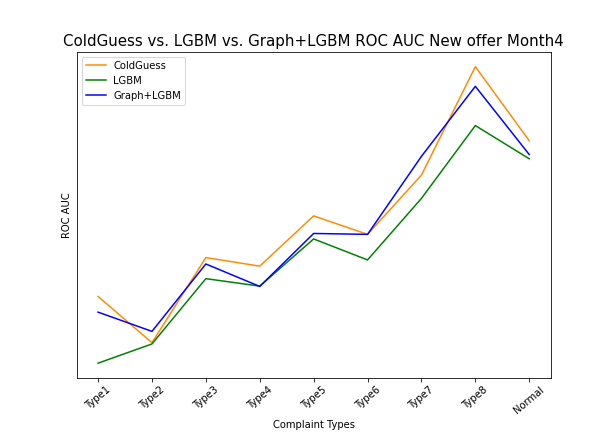}\hfill
    \\[\smallskipamount]
    \includegraphics[width=.35\textwidth]{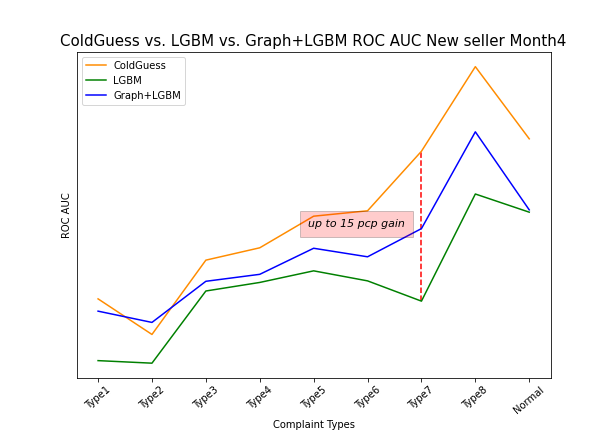}\hfill
    \includegraphics[width=.35\textwidth]{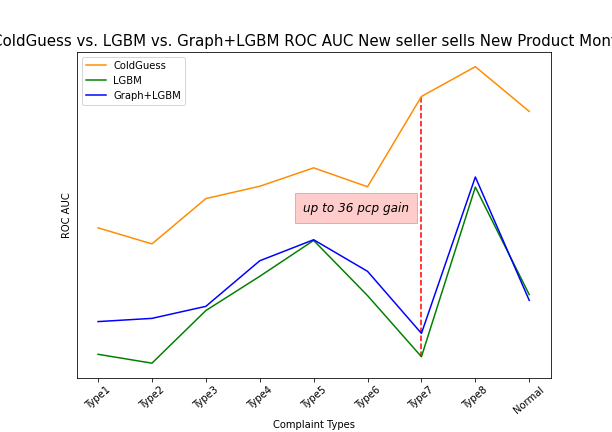}\hfill
    \caption{\method vs. LGBM on a full spectrum of sample data (top left), new offer case (top right), new seller case (bottom left), and new seller sell new ASIN case (bottom right) using data of Month4.}
    \label{fig:202102}
\end{figure*}

\begin{figure*}
    \includegraphics[width=.35\textwidth]{Figures/2021-03_All Data.png}\hfill
    \includegraphics[width=.35\textwidth]{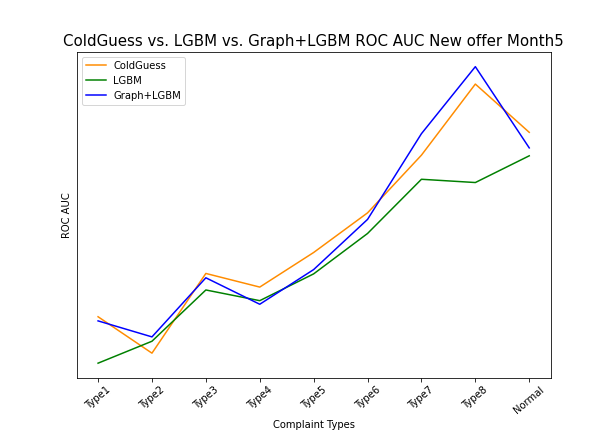}\hfill
    \\[\smallskipamount]
    \includegraphics[width=.35\textwidth]{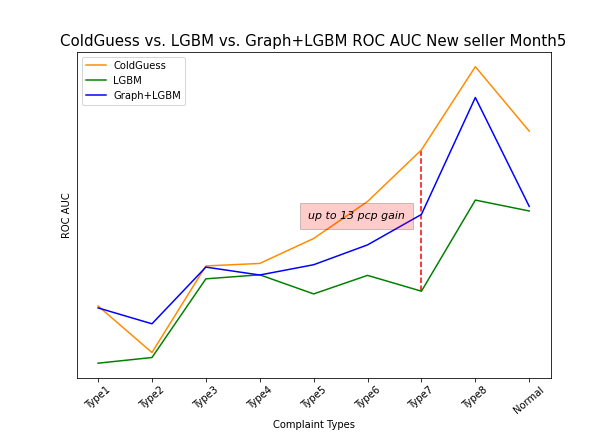}\hfill
    \includegraphics[width=.35\textwidth]{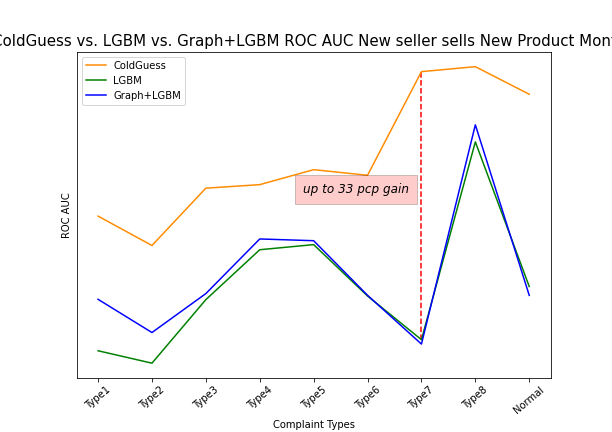}\hfill
    \caption{\method vs. LGBM vs. Graph+LGBM on a full spectrum of sample data (top left), new offer case (top right), new seller case (bottom left), and new seller sell new \ASIN case (bottom right) using data of Month5.}
    \label{fig:202103}
\end{figure*}

\begin{figure*}
    \includegraphics[width=.35\textwidth]{Figures/2021-04_All Data.png}\hfill
    \includegraphics[width=.35\textwidth]{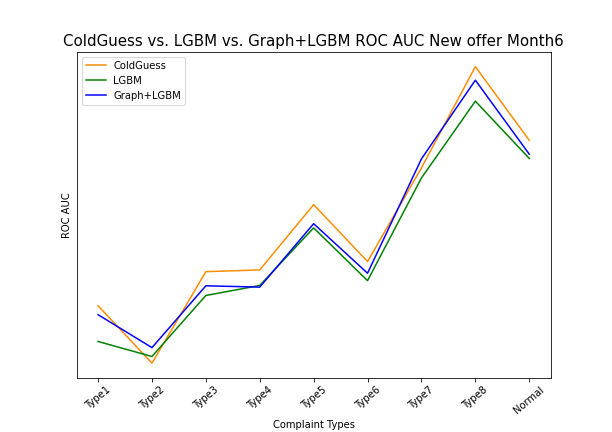}\hfill
    \\[\smallskipamount]
    \includegraphics[width=.35\textwidth]{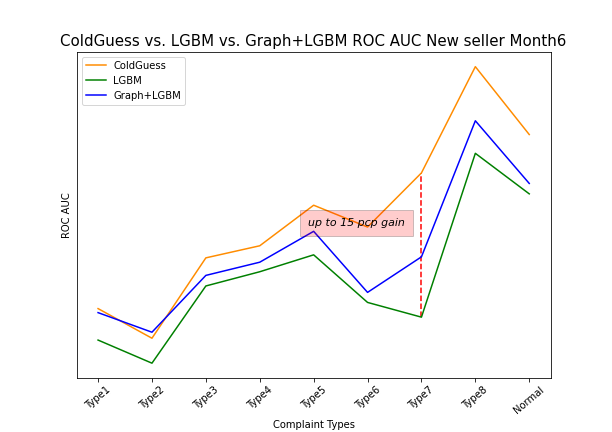}\hfill
    \includegraphics[width=.35\textwidth]{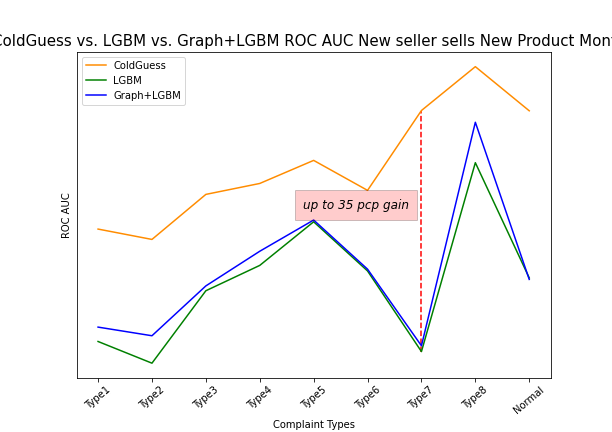}\hfill
    \caption{\method vs. LGBM vs. Graph+LGBM on a full spectrum of sample data (top left), new offer case (top right), new seller case (bottom left), and new seller sell new \ASIN case (bottom right) using data of Month6.}
    \label{fig:202104}
\end{figure*}
